# Supplementary material for: Relaxed Clustered Hawkes Process for Procrastination Modeling in MOOCs
Source: arXiv:2102.00093 source file (2021-01-29)
Supplement: Supplementary file 1 [file appendix.tex]

\input{AuthorKit21/supplementary/intuition}
\input{AuthorKit21/supplementary/algorithm}
